# Supplementary material for: Transferring Clinical Knowledge into ECGs Representation
Source: arXiv:2512.07021 source file (2025-12-07)
Supplement: Supplementary file 1 [file appendix.tex]

% \appendix
% \section*{Appendix}

% \section{Detailed Classification Analysis}
% here we have the metrics for each diagnoses leveraging \{code chapters, condition prevalence, etc\}

% \section{Detailed Estimation Analysis}
% same thing but for lab abnormalities
